# Supplementary material for: Energetics of H$_2$ clusters from density functional and coupled cluster theories
Source: arXiv:1611.00371 source file (2016-11-01)
Supplement: Supplementary file 1 [file supplementary.pdf]

# Energetics of $H_2$ clusters from density functional and coupled cluster theories: Supplementary Material

J. R. Trail, P. López Ríos, and R. J. Needs
*Theory of Condensed Matter Group, Cavendish Laboratory,*
*J J Thomson Avenue, Cambridge CB3 0HE, United Kingdom*
(Dated: November 1, 2016)

## I. GAUSSIAN BASIS SET ERROR ANALYSIS

In the paper we analyze the convergence of total energies extrapolated to the complete basis set limit using cc-pV$n$Z basis sets[1]. Here we justify limiting our calculations to this class of basis sets and not correcting for the basis set superposition error.

In principle, aug-cc-pV$n$Z basis sets would provide a more accurate description of the long-range interaction between hydrogen molecules in our clusters. To quantify such an improvement, we evaluate coupled cluster singles, doubles, and perturbative triples [CCSD(T)] total energies using aug-cc-pV$n$Z basis sets[1] for clusters with seven hydrogen molecules or fewer. The CBS limit[2] is obtained by "efficient" (TQ) extrapolation, as described in the paper. The resulting total energies differed from those obtained with the cc-pV$n$Z basis sets by less than 1 meV/[$H_2$]. This demonstrates that the cc-pV$n$Z basis sets are sufficiently accurate for our purposes, and that augmentation is not required.

Extrapolation to the CBS limit is inherently imperfect[3], hence some of the basis set superposition error will remain after extrapolation. As a further check of the quality of our extrapolations, we quantify this remnant error by calculating single-molecule total energies (with geometries taken from the $C2/c$-24 structure at 150 GPa) using cc-pV$nz$ basis functions centred on the two atomic sites only, and with additional basis functions at dummy sites associated with the rest of the $H_{24}$ cluster. The resulting energies, obtained using "efficient" (TQ) extrapolation, differ by $-0.69$ and 0.09 meV/[$H_2$] for CCSD(T) and DFT with the B3LYP functional, respectively. This demonstrates that the "efficient extrapolation" procedure does not suffer from significant basis set superposition errors.

## II. DETAILS OF DMC CALCULATIONS

The quantum Monte Carlo[4] calculations reported in the paper are performed using the CASINO code[5]. The trial wave function used in these calculations consists of Slater determinants of cc-pVQZ orbitals produced by the $O_3$ GGA density functional, multiplied by a Jastrow correlation factor of the Drummond-Towler-Needs form[6,7] containing electron-electron, electron-nucleus and electron-electron-nucleus terms with a total of 76 variable parameters. The Gaussian orbitals are cusp-corrected[8] to prevent divergences of the local energy at electron-nucleus coalescence points. We use linear least-squares energy minimization[9,10] to optimize the parameters in the Jastrow factor at the variational Monte Carlo level.

We conduct an initial convergence survey to determine the range of time steps to use in the diffusion Monte Carlo (DMC) calculations by performing DMC runs at several time steps in the range 0.001–0.2 a.u. for the 6-atom cluster extracted from the $C2/c$-24 structure at a DFT pressure of 250 GPa. This system corresponds to the median value of the minimum interatomic distance of all the clusters in our DMC calculations, and therefore we expect the convergence tests to reasonably represent the time-step behavior of the full range of clusters. These DMC calculations are performed with a target population of 1024 walkers and a target statistical uncertainty of 0.8 meV/[$H_2$]. The results of the survey are plotted in Fig. 1, which shows that time-step dependence is negligible compared with the statistical uncertainty for time steps of up to 0.1 a.u.

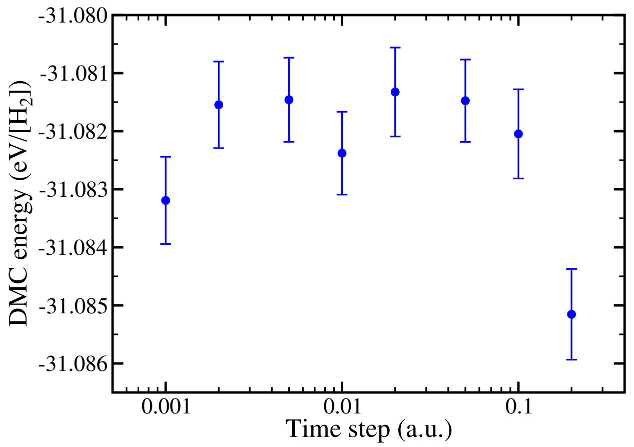


FIG. 1. DMC energy as a function of time step for the 6-atom cluster extracted from the bulk $C2/c$-24 structure at a DFT pressure of 250 GPa, using a target population of 1024 walkers. Note the logarithmic scale on the horizontal axis.

The production DMC calculations are carried out using time steps of 0.005 and 0.02 a.u. with respective target populations of 4096 and 1024 walkers, allowing simultaneous extrapolation of the DMC energies to zero time step and infinite population from the two DMC calculations. The numbers of Monte Carlo steps are chosen so as to minimize the computational cost of the calculations[11] and to obtain the final DMC energies with a statistical

uncertainty of 1.0 meV/[$H_2$] or less.

## III. BULK HYDROGEN GEOMETRIES

The bulk geometries from which the hydrogen clusters are extracted are provided below. Table I contains unit cell parameters for the 5 symmetries and 3 pressures considered. Tables II–XVI give the positions of the hydrogen atoms in fractional coordinates for each of the 15 crystalline systems.

| Structure | $p$ (GPa) | Vector | $x$ (Å) | $y$ (Å) | $z$ (Å) |
|---|---|---|---|---|---|
| $C2/c$-24 | 150 | $\mathbf{a}_1$ | 1.5566154168 | 0.0013821635 | −2.6920910778 |
| | | $\mathbf{a}_2$ | −0.0124463698 | 5.5428412800 | 0.0000000000 |
| | | $\mathbf{a}_3$ | 1.5566154168 | 0.0013821635 | 2.6920910778 |
| | 250 | $\mathbf{a}_1$ | 1.4543364180 | 0.0002235063 | −2.5140573111 |
| | | $\mathbf{a}_2$ | −0.0154060201 | 5.1543835193 | 0.0000000000 |
| | | $\mathbf{a}_3$ | 1.4543364180 | 0.0002235063 | 2.5140573111 |
| | 350 | $\mathbf{a}_1$ | 1.3894516606 | −0.0003290588 | −2.4019611675 |
| | | $\mathbf{a}_2$ | −0.0166319815 | 4.9116059894 | 0.0000000000 |
| | | $\mathbf{a}_3$ | 1.3894516606 | −0.0003290588 | 2.4019611675 |
| $Cmca$-12 | 150 | $\mathbf{a}_1$ | 1.4101440714 | −2.6125983365 | 0.0000000000 |
| | | $\mathbf{a}_2$ | 1.4101440714 | 2.6125983365 | 0.0000000000 |
| | | $\mathbf{a}_3$ | 0.0000000000 | 0.0000000000 | 3.1355634559 |
| | 250 | $\mathbf{a}_1$ | 1.3130898531 | −2.4355880825 | 0.0000000000 |
| | | $\mathbf{a}_2$ | 1.3130898531 | 2.4355880825 | 0.0000000000 |
| | | $\mathbf{a}_3$ | 0.0000000000 | 0.0000000000 | 2.9360260163 |
| | 350 | $\mathbf{a}_1$ | 1.2479663701 | −2.3229381257 | 0.0000000000 |
| | | $\mathbf{a}_2$ | 1.2479663701 | 2.3229381257 | 0.0000000000 |
| | | $\mathbf{a}_3$ | 0.0000000000 | 0.0000000000 | 2.8162227387 |
| $Cmca$-4 | 150 | $\mathbf{a}_1$ | 0.9113042466 | −1.5011203377 | 0.0000000000 |
| | | $\mathbf{a}_2$ | 0.9113042466 | 1.5011203377 | 0.0000000000 |
| | | $\mathbf{a}_3$ | 0.0000000000 | 0.0000000000 | 2.7934860043 |
| | 250 | $\mathbf{a}_1$ | 0.8382055336 | −1.4323622345 | 0.0000000000 |
| | | $\mathbf{a}_2$ | 0.8382055336 | 1.4323622345 | 0.0000000000 |
| | | $\mathbf{a}_3$ | 0.0000000000 | 0.0000000000 | 2.5839625621 |
| | 350 | $\mathbf{a}_1$ | 0.7969880090 | −1.3829038688 | 0.0000000000 |
| | | $\mathbf{a}_2$ | 0.7969880090 | 1.3829038688 | 0.0000000000 |
| | | $\mathbf{a}_3$ | 0.0000000000 | 0.0000000000 | 2.4552586432 |
| $P2_1c$-24 | 150 | $\mathbf{a}_1$ | 8.4489079508 | 0.0000000000 | 0.0052181483 |
| | | $\mathbf{a}_2$ | 0.0000000000 | 1.7962169695 | 0.0000000000 |
| | | $\mathbf{a}_3$ | −5.6324823127 | 0.0000000000 | 3.0989898465 |
| | 250 | $\mathbf{a}_1$ | 7.8260521820 | 0.0000000000 | 0.0210840941 |
| | | $\mathbf{a}_2$ | 0.0000000000 | 1.6774497067 | 0.0000000000 |
| | | $\mathbf{a}_3$ | −5.2112852293 | 0.0000000000 | 2.8872234456 |
| | 350 | $\mathbf{a}_1$ | 7.3641791007 | 0.0000000000 | 0.0642838073 |
| | | $\mathbf{a}_2$ | 0.0000000000 | 1.5967185567 | 0.0000000000 |
| | | $\mathbf{a}_3$ | −4.8874492875 | 0.0000000000 | 2.7331023966 |
| $Pc$-48 | 150 | $\mathbf{a}_1$ | 3.1049412941 | 0.0000000000 | 0.0015626262 |
| | | $\mathbf{a}_2$ | 0.0000000000 | 5.4009210140 | 0.0000000000 |
| | | $\mathbf{a}_3$ | −0.0114387929 | 0.0000000000 | 5.5497264133 |
| | 250 | $\mathbf{a}_1$ | 2.8953306324 | 0.0000000000 | −0.0000091951 |
| | | $\mathbf{a}_2$ | 0.0000000000 | 5.0364496526 | 0.0000000000 |
| | | $\mathbf{a}_3$ | −0.0132809057 | 0.0000000000 | 5.1727865990 |
| | 350 | $\mathbf{a}_1$ | 2.7645498755 | 0.0000000000 | −0.0010251315 |
| | | $\mathbf{a}_2$ | 0.0000000000 | 4.8101136482 | 0.0000000000 |
| | | $\mathbf{a}_3$ | −0.0144984358 | 0.0000000000 | 4.9368897741 |

TABLE I. Unit cells for the 5 bulk hydrogen structures at DFT pressures of 150, 250, and 350 GPa.

| $i$ | $f_1^{(i)}$ | $f_2^{(i)}$ | $f_3^{(i)}$ |
|---|---|---|---|
| 1 | 0.844298061322166 | 0.120536069414405 | 0.500939732810289 |
| 2 | 0.155701938677834 | 0.879463930585594 | 0.499060267189709 |
| 3 | 0.999060267189709 | 0.379463930585595 | 0.655701938677834 |
| 4 | 0.000939732810291 | 0.620536069414406 | 0.344298061322166 |
| 5 | 0.614760216345303 | 0.110842181788245 | 0.520925954730935 |
| 6 | 0.385239783654696 | 0.889157818211756 | 0.479074045269065 |
| 7 | 0.979074045269065 | 0.389157818211756 | 0.885239783654697 |
| 8 | 0.020925954730936 | 0.610842181788244 | 0.114760216345306 |
| 9 | 0.310279829461564 | 0.125654143128265 | 0.757106285888872 |
| 10 | 0.689720170538435 | 0.874345856871731 | 0.242893714111127 |
| 11 | 0.742893714111128 | 0.374345856871732 | 0.189720170538437 |
| 12 | 0.257106285888871 | 0.625654143128269 | 0.810279829461565 |
| 13 | 0.338859666596721 | 0.124764178785196 | 0.009553553520715 |
| 14 | 0.661140333403285 | 0.875235821214801 | 0.990446446479286 |
| 15 | 0.490446446479286 | 0.375235821214804 | 0.161140333403280 |
| 16 | 0.509553553520715 | 0.624764178785199 | 0.838859666596715 |
| 17 | 0.817383958339681 | 0.129067911276366 | 0.993799703387330 |
| 18 | 0.182616041660319 | 0.870932088723634 | 0.006200296612665 |
| 19 | 0.506200296612668 | 0.370932088723634 | 0.682616041660319 |
| 20 | 0.493799703387336 | 0.629067911276366 | 0.317383958339681 |
| 21 | 0.072475495994137 | 0.139140391945957 | 0.214732486959477 |
| 22 | 0.927524504005866 | 0.860859608054043 | 0.785267513040522 |
| 23 | 0.285267513040522 | 0.360859608054042 | 0.427524504005863 |
| 24 | 0.714732486959478 | 0.639140391945957 | 0.572475495994134 |

TABLE II. Fractional coordinates of the hydrogen atoms in the primitive cell of the $C2/c$-24 structure at a DFT pressure of 150 GPa. The Cartesian coordinates of the $i$th atom are $\mathbf{r}_i = \sum_j f_j^{(i)} \mathbf{a}_j$.

| $i$ | $f_1^{(i)}$ | $f_2^{(i)}$ | $f_3^{(i)}$ |
|---|---|---|---|
| 1 | 0.864352383872417 | 0.121468154241467 | 0.500132385110741 |
| 2 | 0.135647616127584 | 0.878531845758533 | 0.499867614889258 |
| 3 | 0.999867614889257 | 0.378531845758533 | 0.635647616127583 |
| 4 | 0.000132385110742 | 0.621468154241467 | 0.364352383872417 |
| 5 | 0.616595409245835 | 0.110447440273497 | 0.521741029014508 |
| 6 | 0.383404590754163 | 0.889552559726504 | 0.478258970985492 |
| 7 | 0.978258970985492 | 0.389552559726504 | 0.883404590754165 |
| 8 | 0.021741029014509 | 0.610447440273496 | 0.116595409245839 |
| 9 | 0.309935298915803 | 0.125981078029336 | 0.757188695769448 |
| 10 | 0.690064701084195 | 0.874018921970660 | 0.242811304230551 |
| 11 | 0.742811304230552 | 0.374018921970661 | 0.190064701084197 |
| 12 | 0.257188695769447 | 0.625981078029340 | 0.809935298915805 |
| 13 | 0.338693010234353 | 0.124612649772657 | 0.028930428900215 |
| 14 | 0.661306989765653 | 0.875387350227339 | 0.971069571099786 |
| 15 | 0.471069571099786 | 0.375387350227343 | 0.161306989765648 |
| 16 | 0.528930428900215 | 0.624612649772661 | 0.838693010234347 |
| 17 | 0.797813149296509 | 0.128177836716121 | 0.972633980911405 |
| 18 | 0.202186850703491 | 0.871822163283879 | 0.027366019088591 |
| 19 | 0.527366019088595 | 0.371822163283880 | 0.702186850703491 |
| 20 | 0.472633980911410 | 0.628177836716121 | 0.297813149296509 |
| 21 | 0.071713146834778 | 0.139352703056712 | 0.213070161763300 |
| 22 | 0.928286853165225 | 0.860647296943288 | 0.786929838236700 |
| 23 | 0.286929838236699 | 0.360647296943288 | 0.428286853165223 |
| 24 | 0.713070161763300 | 0.639352703056712 | 0.571713146834775 |

TABLE III. Fractional coordinates of the hydrogen atoms in the primitive cell of the $C2/c$-24 structure at a DFT pressure of 250 GPa. The Cartesian coordinates of the $i$th atom are $\mathbf{r}_i = \sum_j f_j^{(i)} \mathbf{a}_j$.

| $i$ | $f_1^{(i)}$ | $f_2^{(i)}$ | $f_3^{(i)}$ |
|---|---|---|---|
| 1 | 0.875667572504300 | 0.122115135426971 | 0.499057244815170 |
| 2 | 0.124332427495701 | 0.877884864573029 | 0.500942755184828 |
| 3 | 0.000942755184828 | 0.377884864573029 | 0.624332427495700 |
| 4 | 0.999057244815172 | 0.622115135426971 | 0.375667572504299 |
| 5 | 0.614796350427498 | 0.111844658889558 | 0.520775733303972 |
| 6 | 0.385203649572500 | 0.888155341110443 | 0.479224266696029 |
| 7 | 0.979224266696028 | 0.388155341110443 | 0.885203649572502 |
| 8 | 0.020775733303972 | 0.611844658889557 | 0.114796350427500 |
| 9 | 0.311004789561448 | 0.126273432457349 | 0.756043866247177 |
| 10 | 0.688995210438550 | 0.873726567542650 | 0.243956133752822 |
| 11 | 0.743956133752823 | 0.373726567542648 | 0.188995210438552 |
| 12 | 0.256043866247176 | 0.626273432457350 | 0.811004789561450 |
| 13 | 0.338987959472802 | 0.124376929769370 | 0.040642092583720 |
| 14 | 0.661012040527204 | 0.875623070230626 | 0.959357907416281 |
| 15 | 0.459357907416281 | 0.375623070230630 | 0.161012040527199 |
| 16 | 0.540642092583720 | 0.624376929769374 | 0.838987959472796 |
| 17 | 0.786783639861428 | 0.127616494214188 | 0.960538596847287 |
| 18 | 0.213216360138572 | 0.872383505785811 | 0.039461403152709 |
| 19 | 0.539461403152713 | 0.372383505785812 | 0.713216360138572 |
| 20 | 0.460538596847292 | 0.627616494214189 | 0.286783639861428 |
| 21 | 0.073177397698240 | 0.137830531440053 | 0.215139781851460 |
| 22 | 0.926822602301762 | 0.862169468559947 | 0.784860218148539 |
| 23 | 0.284860218148539 | 0.362169468559947 | 0.426822602301760 |
| 24 | 0.715139781851461 | 0.637830531440053 | 0.573177397698238 |

TABLE IV. Fractional coordinates of the hydrogen atoms in the primitive cell of the $C2/c$-24 structure at a DFT pressure of 350 GPa. The Cartesian coordinates of the $i$th atom are $\mathbf{r}_i = \sum_j f_j^{(i)} \mathbf{a}_j$.

| $i$ | $f_1^{(i)}$ | $f_2^{(i)}$ | $f_3^{(i)}$ |
|---|---|---|---|
| 1 | 0.999686420210772 | 0.000313579789229 | 0.121842720626789 |
| 2 | 0.500313579789228 | 0.499686420210770 | 0.621842720626786 |
| 3 | 0.000313579789229 | 0.999686420210772 | 0.878157279373214 |
| 4 | 0.499686420210770 | 0.500313579789228 | 0.378157279373210 |
| 5 | 0.866492715858417 | 0.133507284141586 | 0.455577843197975 |
| 6 | 0.633507284141583 | 0.366492715858417 | 0.955577843197978 |
| 7 | 0.133507284141586 | 0.866492715858417 | 0.544422156802022 |
| 8 | 0.366492715858417 | 0.633507284141583 | 0.044422156802024 |
| 9 | 0.745156133383835 | 0.254843866616166 | 0.325862676167131 |
| 10 | 0.754843866616165 | 0.245156133383834 | 0.825862676167132 |
| 11 | 0.254843866616166 | 0.745156133383835 | 0.674137323832868 |
| 12 | 0.245156133383834 | 0.754843866616165 | 0.174137323832869 |

TABLE V. Fractional coordinates of the hydrogen atoms in the primitive cell of the $Cmca$-12 structure at a DFT pressure of 150 GPa. The Cartesian coordinates of the $i$th atom are $\mathbf{r}_i = \sum_j f_j^{(i)} \mathbf{a}_j$.

| $i$ | $f_1^{(i)}$ | $f_2^{(i)}$ | $f_3^{(i)}$ |
|---|---|---|---|
| 1 | 0.997608068367409 | 0.002391931632593 | 0.131747608543182 |
| 2 | 0.502391931632591 | 0.497608068367406 | 0.631747608543179 |
| 3 | 0.002391931632593 | 0.997608068367409 | 0.868252391456821 |
| 4 | 0.497608068367406 | 0.502391931632591 | 0.368252391456817 |
| 5 | 0.867817277816937 | 0.132182722183066 | 0.454187081290956 |
| 6 | 0.632182722183063 | 0.367817277816937 | 0.954187081290960 |
| 7 | 0.132182722183066 | 0.867817277816937 | 0.545812918709040 |
| 8 | 0.367817277816937 | 0.632182722183063 | 0.045812918709042 |
| 9 | 0.735479345000384 | 0.264520654999617 | 0.318428730701838 |
| 10 | 0.764520654999616 | 0.235479345000383 | 0.818428730701839 |
| 11 | 0.264520654999617 | 0.735479345000384 | 0.681571269298161 |
| 12 | 0.235479345000383 | 0.764520654999616 | 0.181571269298162 |

TABLE VI. Fractional coordinates of the hydrogen atoms in the primitive cell of the *Cmca*-12 structure at a DFT pressure of 250 GPa. The Cartesian coordinates of the $i$th atom are $\mathbf{r}_i = \sum_j f_j^{(i)} \mathbf{a}_j$.

| $i$ | $f_1^{(i)}$ | $f_2^{(i)}$ | $f_3^{(i)}$ |
|---|---|---|---|
| 1 | 0.994662060462133 | 0.005337939537869 | 0.138746349343147 |
| 2 | 0.505337939537867 | 0.494662060462130 | 0.638746349343144 |
| 3 | 0.005337939537869 | 0.994662060462133 | 0.861253650656856 |
| 4 | 0.494662060462130 | 0.505337939537867 | 0.361253650656852 |
| 5 | 0.868559651599298 | 0.131440348400705 | 0.453506837811739 |
| 6 | 0.631440348400702 | 0.368559651599298 | 0.953506837811744 |
| 7 | 0.131440348400705 | 0.868559651599298 | 0.546493162188256 |
| 8 | 0.368559651599298 | 0.631440348400702 | 0.046493162188259 |
| 9 | 0.728020039515867 | 0.271979960484134 | 0.314689354703030 |
| 10 | 0.771979960484133 | 0.228020039515866 | 0.814689354703032 |
| 11 | 0.271979960484134 | 0.728020039515867 | 0.685310645296968 |
| 12 | 0.228020039515866 | 0.771979960484133 | 0.185310645296969 |

TABLE VII. Fractional coordinates of the hydrogen atoms in the primitive cell of the *Cmca*-12 structure at a DFT pressure of 350 GPa. The Cartesian coordinates of the $i$th atom are $\mathbf{r}_i = \sum_j f_j^{(i)} \mathbf{a}_j$.

| $i$ | $f_1^{(i)}$ | $f_2^{(i)}$ | $f_3^{(i)}$ |
|---|---|---|---|
| 1 | 0.620938598782534 | 0.379061401217464 | 0.454406395242041 |
| 2 | 0.879061401217466 | 0.120938598782536 | 0.954406395242038 |
| 3 | 0.379061401217464 | 0.620938598782534 | 0.545593604757962 |
| 4 | 0.120938598782536 | 0.879061401217466 | 0.045593604757959 |

TABLE VIII. Fractional coordinates of the hydrogen atoms in the primitive cell of the *Cmca*-4 structure at a DFT pressure of 150 GPa. The Cartesian coordinates of the $i$th atom are $\mathbf{r}_i = \sum_j f_j^{(i)} \mathbf{a}_j$.

| $i$ | $f_1^{(i)}$ | $f_2^{(i)}$ | $f_3^{(i)}$ |
|---|---|---|---|
| 1 | 0.628570765343779 | 0.371429234656218 | 0.448945396172586 |
| 2 | 0.871429234656221 | 0.128570765343782 | 0.948945396172582 |
| 3 | 0.371429234656218 | 0.628570765343779 | 0.551054603827418 |
| 4 | 0.128570765343782 | 0.871429234656221 | 0.051054603827414 |

TABLE IX. Fractional coordinates of the hydrogen atoms in the primitive cell of the *Cmca*-4 structure at a DFT pressure of 250 GPa. The Cartesian coordinates of the $i$th atom are $\mathbf{r}_i = \sum_j f_j^{(i)} \mathbf{a}_j$.

| $i$ | $f_1^{(i)}$ | $f_2^{(i)}$ | $f_3^{(i)}$ |
|---|---|---|---|
| 1 | 0.631262087174260 | 0.368737912825738 | 0.440155540518733 |
| 2 | 0.868737912825740 | 0.131262087174262 | 0.940155540518729 |
| 3 | 0.368737912825738 | 0.631262087174260 | 0.559844459481271 |
| 4 | 0.131262087174262 | 0.868737912825740 | 0.059844459481267 |

TABLE X. Fractional coordinates of the hydrogen atoms in the primitive cell of the $Cmca$-4 structure at a DFT pressure of 350 GPa. The Cartesian coordinates of the $i$th atom are $\mathbf{r}_i = \sum_j f_j^{(i)} \mathbf{a}_j$.

| $i$ | $f_1^{(i)}$ | $f_2^{(i)}$ | $f_3^{(i)}$ |
|---|---|---|---|
| 1 | 0.824827790119511 | 0.703687852915263 | 0.087719002216304 |
| 2 | 0.175172209880489 | 0.203687852915263 | 0.412280997783696 |
| 3 | 0.175172209880489 | 0.296312147084737 | 0.912280997783696 |
| 4 | 0.824827790119511 | 0.796312147084737 | 0.587719002216304 |
| 5 | 0.888960458303615 | 0.408899387417633 | 0.228865388662822 |
| 6 | 0.111039541696385 | 0.908899387417633 | 0.271134611337178 |
| 7 | 0.111039541696385 | 0.591100612582367 | 0.771134611337178 |
| 8 | 0.888960458303615 | 0.091100612582367 | 0.728865388662822 |
| 9 | 0.868975850325337 | 0.149961532550744 | 0.426399945657078 |
| 10 | 0.131024149674663 | 0.649961532550744 | 0.073600054342922 |
| 11 | 0.131024149674663 | 0.850038467449256 | 0.573600054342922 |
| 12 | 0.868975850325337 | 0.350038467449256 | 0.926399945657078 |
| 13 | 0.741676554531255 | 0.901856290403771 | 0.238984592861372 |
| 14 | 0.258323445468745 | 0.401856290403771 | 0.261015407138628 |
| 15 | 0.258323445468745 | 0.098143709596229 | 0.761015407138628 |
| 16 | 0.741676554531255 | 0.598143709596229 | 0.738984592861372 |
| 17 | 0.577766154665325 | 0.362784154028915 | 0.197741735271061 |
| 18 | 0.422233845334675 | 0.862784154028915 | 0.302258264728939 |
| 19 | 0.422233845334675 | 0.637215845971085 | 0.802258264728939 |
| 20 | 0.577766154665325 | 0.137215845971085 | 0.697741735271061 |
| 21 | 0.467192524075626 | 0.620137054369984 | 0.123793830094820 |
| 22 | 0.532807475924374 | 0.120137054369984 | 0.376206169905180 |
| 23 | 0.532807475924374 | 0.379862945630015 | 0.876206169905180 |
| 24 | 0.467192524075626 | 0.879862945630015 | 0.623793830094820 |

TABLE XI. Fractional coordinates of the hydrogen atoms in the primitive cell of the $P2_1c$-24 structure at a DFT pressure of 150 GPa. The Cartesian coordinates of the $i$th atom are $\mathbf{r}_i = \sum_j f_j^{(i)} \mathbf{a}_j$.

| $i$ | $f_1^{(i)}$ | $f_2^{(i)}$ | $f_3^{(i)}$ |
|---|---|---|---|
| 1 | 0.823856687318829 | 0.756842228596225 | 0.080359742727775 |
| 2 | 0.176143312681171 | 0.256842228596224 | 0.419640257272225 |
| 3 | 0.176143312681171 | 0.243157771403775 | 0.919640257272225 |
| 4 | 0.823856687318829 | 0.743157771403777 | 0.580359742727774 |
| 5 | 0.883626062845437 | 0.423937438968198 | 0.220523165438968 |
| 6 | 0.116373937154563 | 0.923937438968199 | 0.279476834561032 |
| 7 | 0.116373937154563 | 0.576062561031802 | 0.779476834561032 |
| 8 | 0.883626062845437 | 0.076062561031802 | 0.720523165438968 |
| 9 | 0.876961617546539 | 0.182223594535322 | 0.432943951310449 |
| 10 | 0.123038382453461 | 0.682223594535320 | 0.067056048689551 |
| 11 | 0.123038382453461 | 0.817776405464678 | 0.567056048689551 |
| 12 | 0.876961617546539 | 0.317776405464678 | 0.932943951310449 |
| 13 | 0.741095006904466 | 0.896873009425202 | 0.242413231291668 |
| 14 | 0.258904993095534 | 0.396873009425202 | 0.257586768708333 |
| 15 | 0.258904993095534 | 0.103126990574798 | 0.757586768708332 |
| 16 | 0.741095006904466 | 0.603126990574797 | 0.742413231291668 |
| 17 | 0.573045677902504 | 0.324312466738279 | 0.192448644942835 |
| 18 | 0.426954322097496 | 0.824312466738278 | 0.307551355057166 |
| 19 | 0.426954322097496 | 0.675687533261721 | 0.807551355057165 |
| 20 | 0.573045677902504 | 0.175687533261721 | 0.692448644942836 |
| 21 | 0.459246527461095 | 0.622875487181663 | 0.114523776551135 |
| 22 | 0.540753472538905 | 0.122875487181659 | 0.385476223448864 |
| 23 | 0.540753472538905 | 0.377124512818337 | 0.885476223448865 |
| 24 | 0.459246527461095 | 0.877124512818339 | 0.614523776551134 |

TABLE XII. Fractional coordinates of the hydrogen atoms in the primitive cell of the $P2_1c$-24 structure at a DFT pressure of 250 GPa. The Cartesian coordinates of the $i$th atom are $\mathbf{r}_i = \sum_j f_j^{(i)} \mathbf{a}_j$.

| $i$ | $f_1^{(i)}$ | $f_2^{(i)}$ | $f_3^{(i)}$ |
|---|---|---|---|
| 1 | 0.825157278081400 | 0.872417515145618 | 0.075856080545983 |
| 2 | 0.174842721918600 | 0.372417515145618 | 0.424143919454017 |
| 3 | 0.174842721918600 | 0.127582484854382 | 0.924143919454017 |
| 4 | 0.825157278081400 | 0.627582484854382 | 0.575856080545983 |
| 5 | 0.860471421698945 | 0.453475309134013 | 0.184723758888063 |
| 6 | 0.139528578301055 | 0.953475309134013 | 0.315276241111937 |
| 7 | 0.139528578301055 | 0.546524690865986 | 0.815276241111937 |
| 8 | 0.860471421698945 | 0.046524690865986 | 0.684723758888063 |
| 9 | 0.883099122350364 | 0.268347240724706 | 0.432403126608498 |
| 10 | 0.116900877649636 | 0.768347240724706 | 0.067596873391502 |
| 11 | 0.116900877649636 | 0.731652759275293 | 0.567596873391502 |
| 12 | 0.883099122350364 | 0.231652759275293 | 0.932403126608498 |
| 13 | 0.764136704545968 | 0.879591671660273 | 0.286753072295131 |
| 14 | 0.235863295454032 | 0.379591671660273 | 0.213246927704869 |
| 15 | 0.235863295454032 | 0.120408328339726 | 0.713246927704869 |
| 16 | 0.764136704545968 | 0.620408328339726 | 0.786753072295131 |
| 17 | 0.541885180765101 | 0.230539528857945 | 0.151146306941351 |
| 18 | 0.458114819234899 | 0.730539528857945 | 0.348853693058648 |
| 19 | 0.458114819234899 | 0.769460471142055 | 0.848853693058649 |
| 20 | 0.541885180765101 | 0.269460471142055 | 0.651146306941352 |
| 21 | 0.456824764935394 | 0.610156972489157 | 0.110533474471743 |
| 22 | 0.543175235064606 | 0.110156972489156 | 0.389466525528257 |
| 23 | 0.543175235064606 | 0.389843027510843 | 0.889466525528257 |
| 24 | 0.456824764935394 | 0.889843027510843 | 0.610533474471743 |

TABLE XIII. Fractional coordinates of the hydrogen atoms in the primitive cell of the $P2_1c$-24 structure at a DFT pressure of 350 GPa. The Cartesian coordinates of the $i$th atom are $\mathbf{r}_i = \sum_j f_j^{(i)} \mathbf{a}_j$.

| $i$ | $f_1^{(i)}$ | $f_2^{(i)}$ | $f_3^{(i)}$ |
|---|---|---|---|
| 1 | 0.050072570332766 | 0.122429851284131 | 0.773070719976110 |
| 2 | 0.225497345975452 | 0.209964362751781 | 0.748943268294109 |
| 3 | 0.226651115173282 | 0.553266723612032 | 0.736522474755518 |
| 4 | 0.685639262184803 | 0.166359053273079 | 0.993882580684140 |
| 5 | 0.979052962016134 | 0.307690097571784 | 0.989009268553196 |
| 6 | 0.883165413543389 | 0.437973033555443 | 0.993801146954406 |
| 7 | 0.733709000630749 | 0.384728077713707 | 0.247780795332399 |
| 8 | 0.571505608932781 | 0.289488600660633 | 0.274286345268189 |
| 9 | 0.573747788669858 | 0.952685645401142 | 0.258003606350050 |
| 10 | 0.946581412496215 | 0.320211388226963 | 0.490522436424632 |
| 11 | 0.868156632047690 | 0.103726516669875 | 0.489841434774559 |
| 12 | 0.017267462602280 | 0.991906779410513 | 0.499817746758222 |
| 13 | 0.236061107087803 | 0.112690517409614 | 0.225899389691365 |
| 14 | 0.072363994979715 | 0.210612007398663 | 0.229450585512917 |
| 15 | 0.073262259613107 | 0.548113427335352 | 0.250942716472477 |
| 16 | 0.440998802101535 | 0.182051683523879 | 0.994804063708851 |
| 17 | 0.376542806362775 | 0.399029591822326 | 0.995648448798736 |
| 18 | 0.521508740021821 | 0.513243971375159 | 0.993363449762200 |
| 19 | 0.555387134310476 | 0.377085386042452 | 0.742296942489385 |
| 20 | 0.727678733684919 | 0.289113015808084 | 0.712381396063032 |
| 21 | 0.722655091280497 | 0.946737842130884 | 0.730987577061928 |
| 22 | 0.190399362944249 | 0.338284480579329 | 0.494586906639326 |
| 23 | 0.476116061952278 | 0.189314987140465 | 0.499429612384971 |
| 24 | 0.376320331055439 | 0.060085660913451 | 0.494491087289278 |
| 25 | 0.050072570332766 | 0.877570148715870 | 0.273070719976111 |
| 26 | 0.225497345975452 | 0.790035637248219 | 0.248943268294110 |
| 27 | 0.226651115173282 | 0.446733276387967 | 0.236522474755518 |
| 28 | 0.685639262184803 | 0.833640946726921 | 0.493882580684141 |
| 29 | 0.979052962016134 | 0.692309902428219 | 0.489009268553196 |
| 30 | 0.883165413543389 | 0.562026966444555 | 0.493801146954408 |
| 31 | 0.733709000630749 | 0.615271922286290 | 0.747780795332399 |
| 32 | 0.571505608932781 | 0.710511399339367 | 0.774286345268192 |
| 33 | 0.573747788669858 | 0.047314354598859 | 0.758003606350051 |
| 34 | 0.946581412496215 | 0.679788611773036 | 0.990522436424632 |
| 35 | 0.868156632047690 | 0.896273483330127 | 0.989841434774561 |
| 36 | 0.017267462602280 | 0.008093220589491 | 0.999817746758222 |
| 37 | 0.236061107087803 | 0.887309482590386 | 0.725899389691364 |
| 38 | 0.072363994979715 | 0.789387992601337 | 0.729450585512917 |
| 39 | 0.073262259613107 | 0.451886572664647 | 0.750942716472477 |
| 40 | 0.440998802101535 | 0.817948316476121 | 0.494804063708851 |
| 41 | 0.376542806362775 | 0.600970408177675 | 0.495648448798735 |
| 42 | 0.521508740021821 | 0.486756028624841 | 0.493363449762199 |
| 43 | 0.555387134310476 | 0.622914613957546 | 0.242296942489386 |
| 44 | 0.727678733684919 | 0.710886984191916 | 0.212381396063031 |
| 45 | 0.722655091280497 | 0.053262157869117 | 0.230987577061928 |
| 46 | 0.190399362944249 | 0.661715519420672 | 0.994586906639325 |
| 47 | 0.476116061952278 | 0.810685012859533 | 0.999429612384971 |
| 48 | 0.376320331055439 | 0.939914339086551 | 0.994491087289278 |

TABLE XIV. Fractional coordinates of the hydrogen atoms in the primitive cell of the $Pc$-48 structure at a DFT pressure of 150 GPa. The Cartesian coordinates of the $i$th atom are $\mathbf{r}_i = \sum_j f_j^{(i)} \mathbf{a}_j$.

| $i$ | $f_1^{(i)}$ | $f_2^{(i)}$ | $f_3^{(i)}$ |
|---|---|---|---|
| 1 | 0.049436525563391 | 0.118776439416637 | 0.775605736785149 |
| 2 | 0.230824293135293 | 0.213387872725197 | 0.745373168723861 |
| 3 | 0.231347548818700 | 0.553727399792433 | 0.733390132264120 |
| 4 | 0.732299242170128 | 0.166533610255467 | 0.994254349370619 |
| 5 | 0.968827713218277 | 0.314051661058593 | 0.990598738056629 |
| 6 | 0.860858879677255 | 0.461448343511953 | 0.994082227145772 |
| 7 | 0.737984718578148 | 0.385478160364606 | 0.245397862541975 |
| 8 | 0.563392768784894 | 0.285966094167731 | 0.274443570170491 |
| 9 | 0.567051289165721 | 0.949203098671704 | 0.259753327530388 |
| 10 | 0.962511921436999 | 0.319046069386700 | 0.491136726654493 |
| 11 | 0.843558311031392 | 0.126685915602712 | 0.491026884166178 |
| 12 | 0.011327967727982 | 0.001471236410613 | 0.499120307666221 |
| 13 | 0.240104096413895 | 0.111004312274055 | 0.221477762899606 |
| 14 | 0.066629270164901 | 0.214071962437998 | 0.235850140488383 |
| 15 | 0.065882605487167 | 0.552317903247556 | 0.253633538197004 |
| 16 | 0.456793601980834 | 0.185271611191251 | 0.994803684520138 |
| 17 | 0.352233037915623 | 0.376265575594612 | 0.994790457206337 |
| 18 | 0.517884552871232 | 0.504830316557915 | 0.993867162192442 |
| 19 | 0.555534323105033 | 0.381866162312068 | 0.744325394746456 |
| 20 | 0.732037004833129 | 0.284811695869424 | 0.711396550621646 |
| 21 | 0.729133440933287 | 0.945943165721809 | 0.729752496450942 |
| 22 | 0.236468207889610 | 0.339147373252599 | 0.493615274044779 |
| 23 | 0.463657491927820 | 0.182135799978954 | 0.498693630935290 |
| 24 | 0.354562187169298 | 0.036603560381652 | 0.493374876621079 |
| 25 | 0.049436525563391 | 0.881223560583364 | 0.275605736785149 |
| 26 | 0.230824293135293 | 0.786612127274803 | 0.245373168723861 |
| 27 | 0.231347548818700 | 0.446272600207567 | 0.233390132264120 |
| 28 | 0.732299242170128 | 0.833466389744533 | 0.494254349370619 |
| 29 | 0.968827713218277 | 0.685948338941407 | 0.490598738056629 |
| 30 | 0.860858879677255 | 0.538551656488047 | 0.494082227145772 |
| 31 | 0.737984718578148 | 0.614521839635394 | 0.745397862541975 |
| 32 | 0.563392768784894 | 0.714033905832269 | 0.774443570170491 |
| 33 | 0.567051289165721 | 0.050796901328297 | 0.759753327530388 |
| 34 | 0.962511921436999 | 0.680953930613299 | 0.991136726654493 |
| 35 | 0.843558311031392 | 0.873314084397288 | 0.991026884166179 |
| 36 | 0.011327967727982 | 0.998528763589388 | 0.999120307666221 |
| 37 | 0.240104096413895 | 0.888995687725945 | 0.721477762899606 |
| 38 | 0.066629270164901 | 0.785928037562002 | 0.735850140488383 |
| 39 | 0.065882605487167 | 0.447682096752444 | 0.753633538197004 |
| 40 | 0.456793601980834 | 0.814728388808749 | 0.494803684520138 |
| 41 | 0.352233037915623 | 0.623734424405388 | 0.494790457206337 |
| 42 | 0.517884552871232 | 0.495169683442085 | 0.493867162192442 |
| 43 | 0.555534323105033 | 0.618133837687931 | 0.244325394746456 |
| 44 | 0.732037004833129 | 0.715188304130575 | 0.211396550621646 |
| 45 | 0.729133440933287 | 0.054056834278191 | 0.229752496450942 |
| 46 | 0.236468207889610 | 0.660852626747401 | 0.993615274044779 |
| 47 | 0.463657491927820 | 0.817864200021046 | 0.998693630935290 |
| 48 | 0.354562187169298 | 0.963396439618348 | 0.993374876621079 |

TABLE XV. Fractional coordinates of the hydrogen atoms in the primitive cell of the $Pc$-48 structure at a DFT pressure of 250 GPa. The Cartesian coordinates of the $i$th atom are $\mathbf{r}_i = \sum_j f_j^{(i)} \mathbf{a}_j$.

| $i$ | $f_1^{(i)}$ | $f_2^{(i)}$ | $f_3^{(i)}$ |
|---|---|---|---|
| 1 | 0.053351572859053 | 0.115744370372635 | 0.773761137338075 |
| 2 | 0.234210565224948 | 0.217803995721737 | 0.739481818204294 |
| 3 | 0.236486951502890 | 0.553567403339784 | 0.730759325547408 |
| 4 | 0.749848762397465 | 0.165596343304413 | 0.993982646624593 |
| 5 | 0.972126608941797 | 0.311200986503992 | 0.992957090850488 |
| 6 | 0.854839238597167 | 0.470296051282183 | 0.994574006955388 |
| 7 | 0.737733126979743 | 0.385894064371492 | 0.241309933998698 |
| 8 | 0.556417320754294 | 0.281926101757060 | 0.270045704004758 |
| 9 | 0.559564539586471 | 0.948596714591970 | 0.261349367975839 |
| 10 | 0.956676136363608 | 0.318766473033787 | 0.491805119639074 |
| 11 | 0.831772258484930 | 0.133370266865270 | 0.492178551097794 |
| 12 | 0.014544497414807 | 0.000666606317732 | 0.498529779887040 |
| 13 | 0.239489446516071 | 0.110977150752996 | 0.219505925011202 |
| 14 | 0.061574612104936 | 0.217188555885907 | 0.245698933613996 |
| 15 | 0.058803711001553 | 0.553211050704280 | 0.256222051862643 |
| 16 | 0.453868689970676 | 0.186298397407778 | 0.994664322502971 |
| 17 | 0.341977333505445 | 0.368749516683924 | 0.992873013494154 |
| 18 | 0.521655757053798 | 0.507403975655366 | 0.993476212368218 |
| 19 | 0.558514410366713 | 0.384763441399327 | 0.746704580330297 |
| 20 | 0.737023745160702 | 0.279525560642199 | 0.717119682036076 |
| 21 | 0.735352951271927 | 0.946342657167754 | 0.728276342086637 |
| 22 | 0.250378461027423 | 0.341823762233745 | 0.493712741313994 |
| 23 | 0.463534150546449 | 0.185327024215686 | 0.497998739756235 |
| 24 | 0.350596152367130 | 0.028614553605168 | 0.492776973500133 |
| 25 | 0.053351572859053 | 0.884255629627365 | 0.273761137338075 |
| 26 | 0.234210565224948 | 0.782196004278263 | 0.239481818204294 |
| 27 | 0.236486951502890 | 0.446432596660216 | 0.230759325547407 |
| 28 | 0.749848762397465 | 0.834403656695586 | 0.493982646624594 |
| 29 | 0.972126608941797 | 0.688799013496008 | 0.492957090850486 |
| 30 | 0.854839238597167 | 0.529703948717818 | 0.494574006955388 |
| 31 | 0.737733126979743 | 0.614105935628508 | 0.741309933998698 |
| 32 | 0.556417320754294 | 0.718073898242940 | 0.770045704004757 |
| 33 | 0.559564539586471 | 0.051403285408032 | 0.761349367975840 |
| 34 | 0.956676136363608 | 0.681233526966213 | 0.991805119639073 |
| 35 | 0.831772258484930 | 0.866629733134730 | 0.992178551097795 |
| 36 | 0.014544497414807 | 0.999333393682269 | 0.998529779887038 |
| 37 | 0.239489446516071 | 0.889022849247004 | 0.719505925011201 |
| 38 | 0.061574612104936 | 0.782811444114093 | 0.745698933613997 |
| 39 | 0.058803711001553 | 0.446788949295719 | 0.756222051862643 |
| 40 | 0.453868689970676 | 0.813701602592223 | 0.494664322502971 |
| 41 | 0.341977333505445 | 0.631250483316076 | 0.492873013494154 |
| 42 | 0.521655757053798 | 0.492596024344632 | 0.493476212368218 |
| 43 | 0.558514410366713 | 0.615236558600673 | 0.246704580330297 |
| 44 | 0.737023745160702 | 0.720474439357801 | 0.217119682036077 |
| 45 | 0.735352951271927 | 0.053657342832247 | 0.228276342086637 |
| 46 | 0.250378461027423 | 0.658176237766254 | 0.993712741313994 |
| 47 | 0.463534150546449 | 0.814672975784315 | 0.997998739756235 |
| 48 | 0.350596152367130 | 0.971385446394831 | 0.992776973500133 |

TABLE XVI. Fractional coordinates of the hydrogen atoms in the primitive cell of the $Pc$-48 structure at a DFT pressure of 350 GPa. The Cartesian coordinates of the $i$th atom are $\mathbf{r}_i = \sum_j f_j^{(i)} \mathbf{a}_j$.

[1] T. H. Dunning Jr., J. Chem. Phys. **90**, 1007 (1989); R. K. Kendall, T. H. Dunning, and R. J. Harrison, J. Chem. Phys. **96**, 6796 (1992).
[2] D. Feller, J. Chem. Phys. **138**, 074103 (2013).
[3] D. S. Ranasinghe and G. A. Petersson, J. Chem. Phys. **138**, 144104 (2013).
[4] W. M. C. Foulkes, L. Mitas, R. J. Needs, and G. Rajagopal, Rev. Mod. Phys. **73**, 33 (2001).
[5] R. J. Needs, M. D. Towler, N. D. Drummond, and P. López Ríos, J. Phys.: Condens. Matter **22**, 023201 (2010).
[6] N. D. Drummond, M. D. Towler, and R. J. Needs, Phys. Rev. B **70**, 235119 (2004).
[7] P. López Ríos, P. Seth, N. D. Drummond, and R. J. Needs, Phys. Rev. E **86**, 036703 (2012).
[8] A. Ma, M. D. Towler, N. D. Drummond, and R. J. Needs, J. Chem. Phys. **122**, 224322 (2005).
[9] C. J. Umrigar, J. Toulouse, C. Filippi, S. Sorella and R. G. Hennig, Phys. Rev. Lett. **98**, 110201 (2007).
[10] J. Toulouse and C. J. Umrigar, J. Chem. Phys. **126**, 084102 (2007).
[11] R. M. Lee, G. J. Conduit, N. Nemec, P. López Ríos, and N. D. Drummond, Phys. Rev. E **83**, 066706 (2011).
